# Supplementary material for: Multi-Center Magnon Excitations Open the Entire Brillouin Zone to Terahertz Magnetometry of Quantum Magnets
Source: arXiv:2203.04343 source file (2022-03-08)
Supplement: Supplementary file 1 [file supplement.pdf]

# Supporting Information

## Multi-Center Magnon Excitations Open the Entire Brillouin Zone to Terahertz Magnetometry of Quantum Magnets

*Tobias Biesner, Seulki Roh, Aleksandar Razpopov, Jannis Willwater, Stefan Süllow, Ying Li, Katharina M. Zoch, Marisa Medarde, Jürgen Nuss, Denis Gorbunov, Yurii Skourski, Andrej Pustogow, Stuart E. Brown, Cornelius Krellner, Roser Valentí, Pascal Puphal, Martin Dressel*

## Contents

**1 Crystal growth** **2**

**2 X-ray diffraction** **3**

**3 ESR measurements** **4**

**4 High-field magnetization** **5**

**5 AC magnetization** **7**

**6 Far-infrared phonons** **8**

**7 Details of the phonon calculations** **9**

**8 Extended data of THz-TDS** **9**

**9 Determination of $\chi''_m$** **10**

**10 THz frequency-domain measurements** **12**

**11 Magneto-optical THz-TDS** **13**

**12 Details of the linear spin-wave theory calculations** **14**

**13 Linear spin-wave theory calculations over an extended energy range** **15**

**14 Calculation of $\chi''_m$** **16**

**15 Linear spin-wave theory calculations under magnetic field** **17**

**16 Two-center magnon and three-center magnon excitation** **19**

**17 Comparison with Herbertsmithite** **20**

# 1 Crystal growth

The crystal growth of $Y_3Cu_9(OH)_{19}Cl_8$ was originally reported in Reference,[1] where 0.59 g $Y_2O_3$, 0.82 g CuO, and 0.89 g $CuCl_2{\cdot}2(H_2O)$ in 10 ml $H_2O$ were heated up to the dissolution point of $Y_2O_3$, followed by a slow cooling to crystallize as sketched in **Figure S1**a. However, these crystals of an average size of 1 x 1 x 1 $mm^3$ suffered from small CuO inclusions since the growth takes place on the surface of the polycrystalline CuO starting material, as the dissolution point of $Y_2O_3$ and the crystallization point of the compound lie above the maximum in solubility of CuO. We thus optimized the synthesis via a horizontal external gradient growth method in a thick-walled quartz ampule by slowly dissolving CuO in a $YCl_3$-$H_2O$ solution and transporting it to the cold end as depicted in Figure S1b. Here, the inclusion free hexagonal single crystals have an average size of 3 x 3 x 1 $mm^3$ up to 3 x 3 x 3 $mm^3$, if grown over several weeks. The pictures of a single crystalline Y-kapellasite are displayed in Figure S1c and d, which show in the given thickness a transparent specimen without any visible impurity inclusions, but some terrace nucleation is apparent.

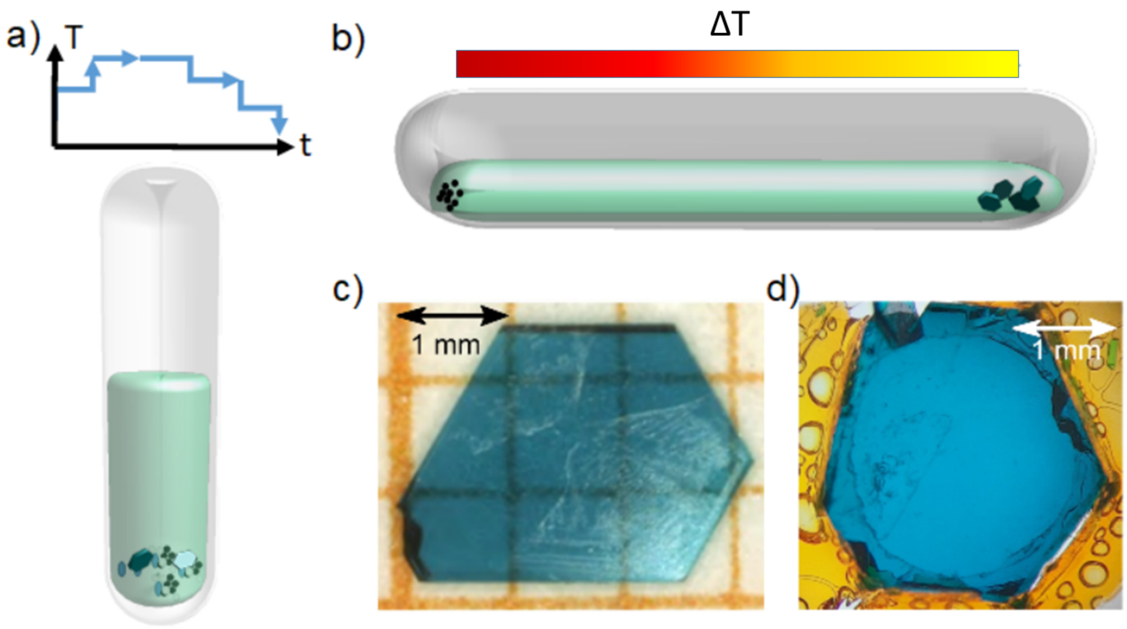


**Figure S1.** Improvement of the growing method of Y-kapellasite. a) Sketch of a thin-walled ampule that is heated and subsequently cooled in an autoclave. b) Sketch of the lying thick-walled quartz ampule that is exposed to an external gradient. Obtained Y-kapellasite single crystals: c) A single crystalline sample of Y-kapellasite with 3 x 3 x 1 $mm^3$ size. d) A sample used in THz-TDS measurements, fixed on the sample holder.

## 2 X-ray diffraction

The structure of $Y_3Cu_9(OH)_{19}Cl_8$ was reported in Reference,[1] while for deuterated powder samples a different result was found in Reference[2] where, in contrast to the single crystal structure, the O1 site has no deuterium leading to the stoichiometry of $Y_3Cu_9(OD)_{18}OCl_8$.
A recent report describes a synthesis of inclusion free crystals using LiOH, $Y(NO_3)_3 \cdot 6H_2O$ and $CuCl_2 \cdot 2H_2O$ with another slightly variated structure, where a partial occupation of Y in the kagome plane is present.[3] This likely presents an example of a phase mixture with $YCu_3(OH)_6Cl_3$.[4] This phase mixture leads to a magnetic transition around 11 K. We note that already the structure solution of $YCu_3(OH)_6Cl_3$ shows a phase mixture as partial occupation of Y out of the kagome plane is observed, which represents structure parts of $Y_3Cu_9(OH)_{19}Cl_8$. For the large inclusion free single crystals, described in our paper, we performed single crystal diffraction to shed light on this various forms of structure. A crystal was broken under high viscosity oil and a 150 $\mu$m piece was mounted with grease on a loop made of Kapton foil (Micromounts, MiTeGen, Ithaca, NY). Diffraction data were collected with a SMART APEX II CCD X-ray diffractometer (Bruker AXS, Karlsruhe, Germany) using graphite-monochromated Mo-$K_\alpha$ radiation ($\lambda = 0.71073$ Å) at low temperature $T = 100(2)$ K. **Figure S2** shows the XRD maps of the (hk0), (h0l), and (0kl) reciprocal lattice planes of the $Y_3Cu_9(OH)_{19}Cl_8$ single crystal. We can confirm the published $Y_3Cu_9(OH)_{19}Cl_8$ structure[1] with a goodness of the fit of 1.1 and find no disorder on the Y site. Note that the crystal under investigation showed reticular-merohedral twinning (reverse-obverse twin). This was taken into account during structure refinement, the twin volume fractions were determined as 0.847(2) and 0.153(2), respectively.

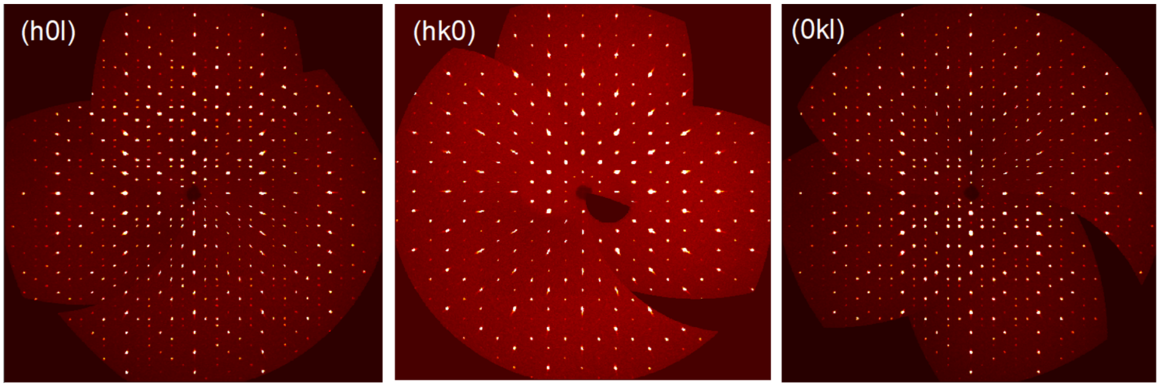


**Figure S2.** Single crystal diffraction. XRD maps of the (h0l), (hk0), and (0kl) planes of the investigated $Y_3Cu_9(OH)_{19}Cl_8$ crystal.

# 3 ESR measurements

Temperature-dependent electron spin resonance (ESR) measurements in the X-band frequency ($f$ = 9.8 GHz) were carried out employing a Bruker (EMXplus) cw-spectrometer and an Oxford Instruments He-flow cryostat. The results are shown in **Figure S3**. The external magnetic field is applied within the kagome planes $\boldsymbol{H} \parallel (a, b)$ and the microwave field $\boldsymbol{h}$ is oriented along the $c$-axis. In Figure S3a, a broad contribution evolves in the derivative of the absorbed microwave power $\mathrm{d}P/\mathrm{d}H$ below the onset of short-range magnetic correlations, $T \approx 30$ K. Further cooling results in a strong increase of the overall amplitude and a shift of the contribution to lower magnetic fields. This broad feature agrees well with the derivative of a Lorentzian (red dashed line). Additional small resonances develop upon cooling, possibly related to tiny magnetic impurities in the sample. The good agreement between the temperature scales of the NMR measurements (see main text) and the ESR investigation suggests short-range magnetic correlations to be the main source of this resonance.

In general, the absorbed microwave power is proportional to the imaginary part of the magnetic susceptibility, $P \propto \chi''$. Hence, $\chi''$ is obtained by integrating the measured derivative of the absorbed power $\mathrm{d}P/\mathrm{d}H$ over the magnetic field $H$ (inset of Figure S3a). The electron spin susceptibility $\chi_s^e$ (Figure S3b, as shown in **Figure 2** of the main text) is directly proportional to the intensity of the ESR absorption line by the Kramers-Kronig sum rule: $\chi_s^e \propto \int_0^\infty P(H)\mathrm{d}H = I$ [5] and therefore obtained from the intensity of the Lorentz fits of $\mathrm{d}P/\mathrm{d}H$.

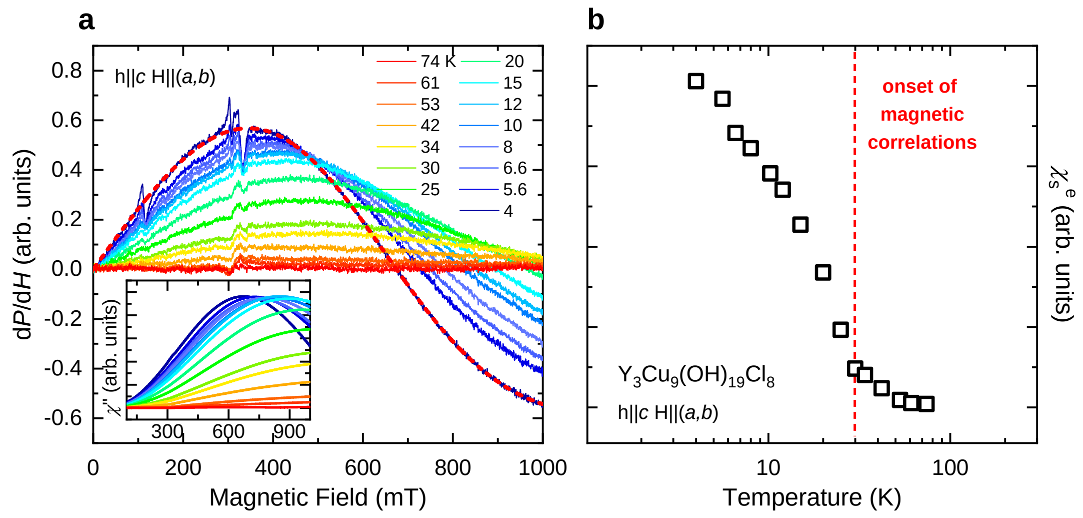


**Figure S3.** X-band ESR measurements of Y-kapellasite. a) Derivative of the absorbed microwave power with respect to the magnetic field: External magnetic field $\boldsymbol{H} \parallel (a, b)$ with microwave field ($f$ = 9.8 GHz) $\boldsymbol{h} \parallel c$. Upon cooling below the onset of short-range magnetic correlations, a large Lorentzian feature starts to develop. Red dashed line: Fit of the Lorentzian derivative for $T$ = 4 K, for example. Inset of (a): $\chi''$ obtained by the integration of $\mathrm{d}P/\mathrm{d}H$. b) Electron spin susceptibility $\chi_s^e$, obtained from the Lorentzian analysis of $\mathrm{d}P/\mathrm{d}H$. A strong increase can be seen at the onset of short-range magnetic correlations (vertical red dashed line).

## 4 High-field magnetization

In order to investigate the low-temperature magnetic transitions further, we performed high-field magnetization measurements. For the measurements with a field parallel to the kagome plane, a single crystal with a total mass of 7.2 mg was aligned in a Laue diffractometer to confirm high crystalline quality. In order to assemble enough material for the configuration with the magnetic field perpendicular to the kagome plane (parallel to the $c$-axis), an array of seven small single crystals with a total weight of 6.8 mg was prepared. The magnetization was measured as a function of temperature and of field up to 5 T with a commercial SQUID-magnetometer. Subsequently, the magnetization was measured at the high field laboratory in Dresden (HLD-EMFL) at temperatures between 0.5 K and 30 K with fields up to 55 T. A coaxial pick-up coil system [6] was used to measure the relative magnetization. Absolute values were scaled by using the data from the SQUID measurements.

The high-field magnetization measurements are presented in **Figure S4**. Above $T = 5$ K the response shows a close-to-linear dependence on the external magnetic field with subtle features developing as the temperature approaches $T_N \approx 2.2$ K. Below $T_N$, a clear magnetization plateau is formed slightly above 15 T, which can be seen in both in-plane and out-of-plane measurements, with plateau values of 0.21 $\mu_B$ for the $a, b$-plane and 0.18 $\mu_B$ for the $c$-axis at $T = 1.5$ K, Figure S4a and c. Increasing the field further, the magnetization rises again by deviating from the plateau response. The differential magnetization (Figure S4b and d) reveals a small change of the slope between 40 to 45 T, suggesting another magnetization plateau with 0.37 $\mu_B$ for the $a, b$-plane and 0.33 $\mu_B$ for the $c$-axis. While the lower field plateaus are robust even in the $^3$He measurements, probing down to $T = 0.49$ K, the more subtle slope changes at high fields are hard to observe here. Considering the similar magnetization for in-plane and out-of-plane orientations, our measurements show that the magnetic anisotropy is rather weak for Y-kapellasite.

The emergence of two plateau-like features at low temperatures around 1/6 and 1/3 of full magnetization suggests an involvement of the spins in the hexagon of the kagome lattice in intermediate magnetic phases before the saturation. Similar observations were made, for instance, in the distorted kagome magnet Volborthite. [7,8]

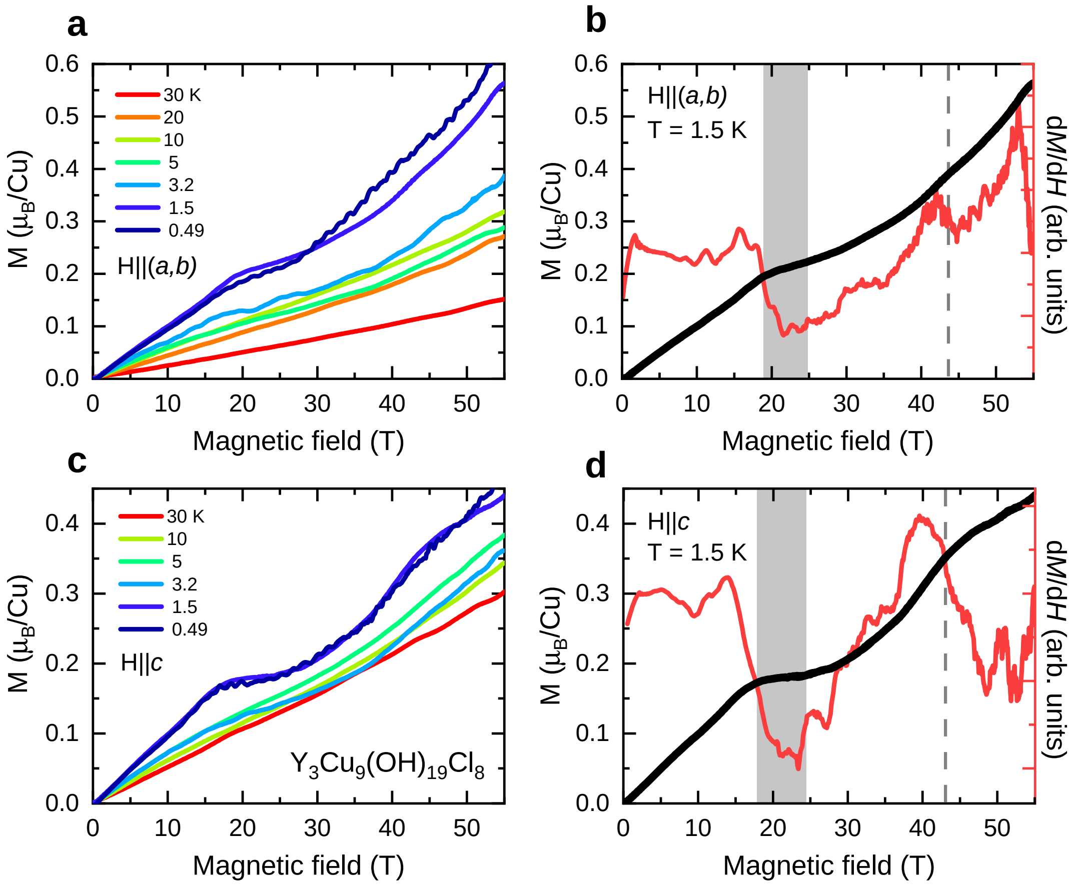


**Figure S4.** Magnetization of Y-kapellasite in pulsed magnetic fields up to **55** T. a) Magnetization $M$ in the $a, b$-plane, $\boldsymbol{H} \parallel (a, b)$. b) Magnetization $M$ (black line, left axis) in comparison to differential magnetization $\mathrm{d}M/\mathrm{d}H$ (red line, right axis) at $T = 1.5$ K. c,d) Results for the c-axis, $\boldsymbol{H} \parallel c$.

## 5 AC magnetization

Dc magnetic susceptibility, shown in the main manuscript, and ac magnetic susceptibility measurements were carried out on these crystals in a range of 0.5–10 K, 0–6 T, and 99–1024 Hz, using a Quantum Design Magnetic Property Measurements System (MPMS) equipped with a $^3$He insert and a Physical Properties Measurement System (PPMS) utilizing the standard ACMS option in the range of 2-300 K, 0-6 T, and 99-9999 Hz. Results are shown in **Figure S5**. With increasing the frequency of the in-plane ac magnetic field of 0.38 mT the imaginary part of the magnetization $M''$ starts to rise, Figure S5a. Reaching a frequency of around 10 kHz, $M''$ shows a broad contribution between 30 K and 100 K, centered at $T = 50$ K, independent of the cooling protocol. Around $T = 2$ K, Figure S5b, a small kink becomes visible for increased frequencies (333-1024 Hz), possibly related to the onset of magnetic ordering. Further cooling results in a strong frequency-dependent behavior. While frequencies below $f = 800$ Hz lead to comparable temperature dependencies, at $f = 1024$ Hz, $M''$ increases below 0.8 K. The enhancement of $M''$ at low temperatures and the broad contribution above $T = 30$ K imply the occurrence of an absorption mechanism for oscillating fields, connected to the long-range magnetic order and the onset of short-range magnetic correlations.

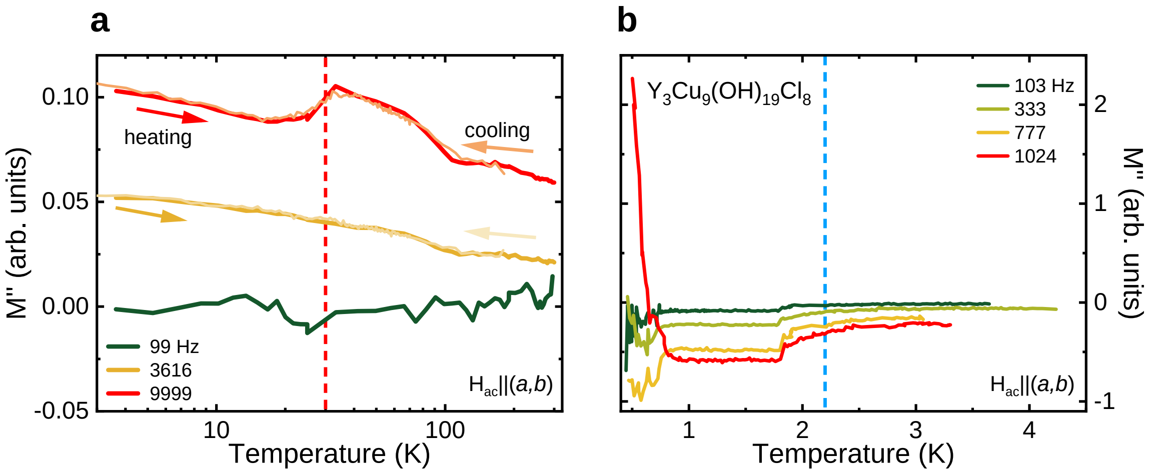


**Figure S5.** AC magnetization of Y-kapellasite. Imaginary part of the magnetization $M''$ with an in-plane oscillating field ($\boldsymbol{H}_{ac} \| (a, b)$) of 0.38 mT for various oscillation frequencies. a) With increasing the frequency, $M''$ starts to rise. The broad contribution between 100 K and 30 might be related to the onset of short-range magnetic correlations (red dashed line), $T \approx 30$ K. b) At low temperatures, $M''$ starts to increase for $f = 1024$ Hz below $T_N = 2.2$ K (blue dashed line).

## 6 Far-infrared phonons

In order to separate the phonon modes from the observed THz response, we performed infrared spectroscopy in an extended frequency range. Far-infrared measurements were carried out in reflection geometry on thick crystals (over 2 mm thickness), using a Bruker 113v FTIR spectrometer equipped with an *in-situ* gold evaporation technique.[9] With the Kramers-Kronig analysis, optical properties are calculated.[10,11] Results in the spectral area of interest are shown in **Figure S6**. Several vibrational modes were observed in both, in-plane and out-of-plane, measurements. With cooling down to $T = 3$ K, most of the phonons show a sharpening and a blueshift, as generally expected. Interesting behavior is observed for the in-plane 80 cm$^{-1}$ feature which exhibits a redshift with cooling, manifesting the negative Grüneisen parameter, i.e. a lattice instability. A magnetoelastic coupling scenario might be possible, similar to the case of Herbertsmithite.[12] A coupling of the phonons and the magnetic texture of Y-kapellasite is indeed corroborated by our magneto-THz results (main text), revealing a shift of the phonon tail of the lowest $E_u$ mode under magnetic field.
Phonon calculations were performed and put in relation to the experimental results. Comparing the observed phonon modes to our calculations, a good agreement of the resonance frequencies is visible, cf. Figure S6a and c. From the density functional theory (DFT) calculations, the two lowest frequency phonon modes are expected to be at 44.9 cm$^{-1}$ ($E_u$) and 47.8 cm$^{-1}$ ($A_u$). In the infrared spectra, these two modes are not well pronounced. However, the phonon tails observed in the THz spectra above 40 cm$^{-1}$ (main text) match well with these frequencies, confirming the influence of phonons at high frequency but not at low frequencies in our THz range.

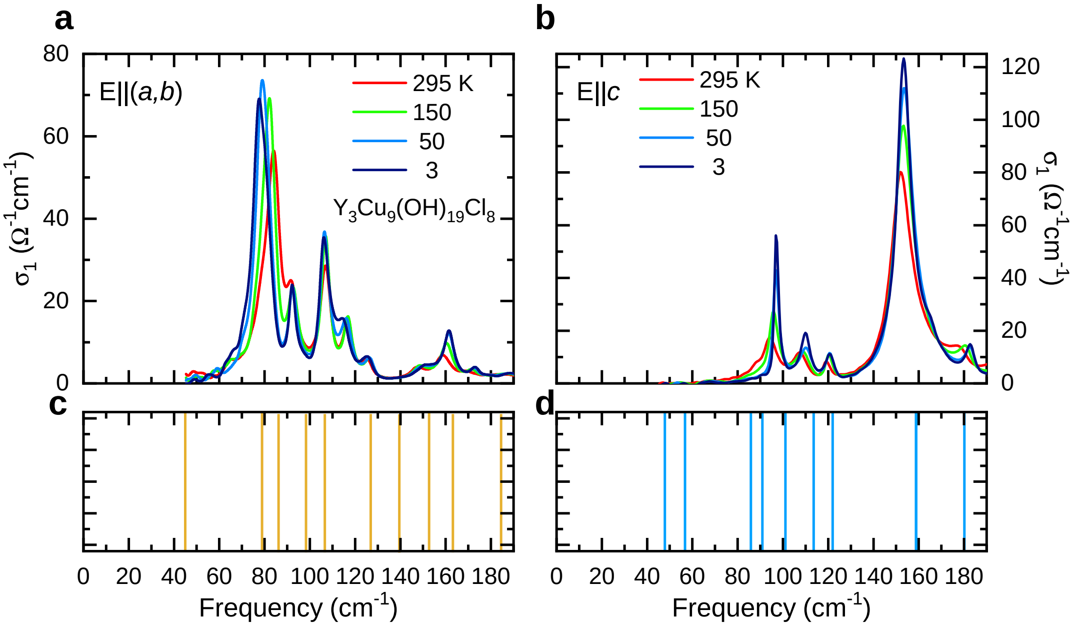


**Figure S6.** Infrared spectra and expected phonon frequencies (DFT calculation). The far-infrared optical conductivity $\sigma_1$ is dominated by multiple phononic contributions: a) in-plane measurements $\boldsymbol{E} \parallel (a, b)$ and b) out-of-plane $\boldsymbol{E} \parallel c$ response. c,d) Calculated $E_u$ and $A_u$ phonon mode frequencies, respectively.

# 7 Details of the phonon calculations

*Ab initio* vibrational studies were performed using the crystal structure of $Y_3Cu_9(OH)_{19}Cl_8$ relaxed from the experimental one at 173 K. [1] In order to keep the symmetry and describe the fractional occupancy of H reported in Reference, [1] we used the virtual crystal approximation (VCA), where we considered fictious 'virtual' atoms that interpolate between the behavior of the H atom and a vacancy. The validity of such an approximation for simulating possible vacancy effects has been tested in the past. [13,14] The phonon frequencies were calculated by diagonalizing the dynamical matrices using the PHONOPY package. [15,16] The dynamical matrices were constructed from the force constants determined from the finite displacements in the conventional unit cell, [17] which is equivalent to three unit cells in Herbertsmithite. [12] The density functional calculations were performed within the Perdew-Burke-Ernzerhof parametrization of the generalized gradient approximation [18] implemented in the Vienna package (VASP). [19,20,21] The Brillouin zone was sampled with a $4 \times 4 \times 4$ k-point mesh, and the plane-wave cutoff was set at 520 eV.

# 8 Extended data of THz-TDS

Temperature-dependent THz-TDS measurements are carried out in transmission geometry employing a Teraview Terapulse 4000 THz-TDS spectrometer along with a He-bath cryostat on oriented single crystals. The time-domain electric fields, which are directly measured from our THz spectrometer, are displayed in **Figure S7**a for in-plane. By performing the Fast Fourier Transformation (FFT), the frequency-dependent power spectrum $\tilde{E}_{sample}(\omega)$ was obtained. Then, the complex transmission $\tilde{Tr}(\omega)$ was calculated by referencing to the empty hole of sample holder, $\tilde{E}_{ref}(\omega)$: $\tilde{Tr}(\omega) = \tilde{E}_{sample}(\omega)/\tilde{E}_{ref}(\omega)$. The absorption coefficient of the sample is related to the transmittance $Tr(\omega)$ (real part of $\tilde{Tr}$) via the Beer-Lambert law: $\alpha(\omega) = -\ln\{Tr(\omega)\}/d$, where $d$ is the thickness of the sample. The absorption coefficient spectra for all measured temperatures are shown in Figure S7b.

The integrated absorption coefficient, which is used to analyze the spectra in the main text, $IA = \int \alpha(\omega)\, \mathrm{d}\omega$ is proportional to the optical spectral weight $SW = \int \sigma(\omega)\, \mathrm{d}\omega$ with the relation $\alpha(\omega) = 4\pi\sigma(\omega)/n(\omega)$, where $\sigma$ is optical conductivity and $n$ is index of refraction. [10,11]

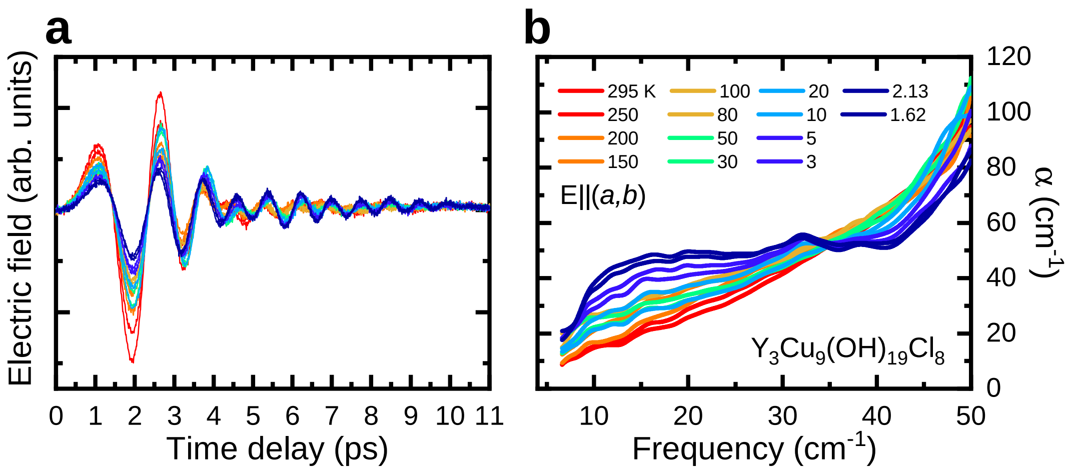


**Figure S7.** THz-TDS result for all measured temperatures. a,b) Time-domain electric field and absorption coefficient for the in-plane $\boldsymbol{E} \parallel (a, b)$ response, respectively.

## 9 Determination of $\chi_m''$

In the main text we show $\chi_m'' = \text{Im}\{\tilde{\chi}_m(\omega)\}$, where $\tilde{\chi}_m(\omega) \approx \frac{2ic}{\sqrt{\tilde{\epsilon}_{ref}}\omega d} \ln\{\frac{\tilde{Tr}_{ref}}{\tilde{Tr}}\}$. Here, the low-temperature magnetic susceptibility $\tilde{\chi}_m$ is extracted from THz-TDS measurements by referencing to the spectra at temperatures above the magnetic ordering (or onset of magnetic interaction). Such an approach was used in References [22, 23, 24, 25, 26, 27] and proven to be robust in the class of insulating quantum magnets since the electronic contributions are located at much higher frequencies. In the following, $\tilde{\chi}_m(\omega)$ is derived using this approach, a more detailed explanation can be found in Reference. [25] In general, complex transmission trough the sample with thickness $d$, can be written as $\tilde{Tr}(\omega) = 4\frac{Z_0\tilde{Z}_s}{(Z_0+\tilde{Z}_s)^2} \exp\{i\frac{\omega d}{c}(\tilde{n}-1)\}$, where $Z_0 = 377\ \Omega$ and $\tilde{Z}_s = \sqrt{\frac{\tilde{\mu}}{\tilde{\epsilon}}}$ is the complex impedance of the sample with permittivity $\tilde{\epsilon}$ and magnetic permeability $\tilde{\mu}$. $\tilde{n} = \sqrt{\tilde{\epsilon}\tilde{\mu}}$ is the index of refraction of the sample. [11, 28] Rewriting the complex transmission in terms of $\tilde{\epsilon}$ and $\tilde{\mu}$ leads to

$$\tilde{Tr}(\omega) = \frac{4\sqrt{\tilde{\epsilon}\tilde{\mu}}}{(\sqrt{\tilde{\epsilon}}+\sqrt{\tilde{\mu}})^2} \exp\{i\frac{\omega d}{c}(\sqrt{\tilde{\epsilon}\tilde{\mu}}-1)\}. \tag{1}$$

For the magnetic permeability we can write $\tilde{\mu} = 1 + \tilde{\chi}_m$. By assuming $\tilde{\chi}_m << 1$ and $\sqrt{\tilde{\mu}} \approx 1 + \tilde{\chi}_m/2$ it reads:

$$\tilde{Tr}(\omega) \approx \frac{4\sqrt{\tilde{\epsilon}}(1+\tilde{\chi}_m/2)}{(\sqrt{\tilde{\epsilon}}+1+\tilde{\chi}_m/2)^2} \exp\{i\frac{\omega d}{c}(\sqrt{\tilde{\epsilon}}(1+\tilde{\chi}_m/2)-1)\}. \tag{2}$$

It can furthermore be simplified as:

$$\tilde{Tr}(\omega) \approx \exp\{i\frac{\omega d}{c}(\sqrt{\tilde{\epsilon}}(1+\tilde{\chi}_m/2)-1)\}, \tag{3}$$

since the exponential term is dominating in Equation 2. To extract $\tilde{\chi}_m$ from Equation 3, the dielectric contribution needs to be subtracted. $\tilde{Tr}$ can be referenced to a temperature, where $\tilde{\mu} \approx 1$, i.e. above the onset of magnetic interactions. Here, the complex transmission reads $\tilde{Tr}_{ref} \approx \exp\{i\frac{\omega d}{c}(\sqrt{\tilde{\epsilon}_{ref}}-1)\}$. Under the assumption that the dielectric properties (phononic or electronic contributions) in the THz range do not change considerably below the reference temperature we can write: $\tilde{\epsilon}_{ref} \approx \tilde{\epsilon}$ and therefore

$\frac{\tilde{T}r}{Tr_{ref}} \approx \exp\{i\frac{\sqrt{\tilde{\epsilon}_{ref}}\omega d}{2c}\tilde{\chi}_m\}$. Inverting this leads to:

$$\tilde{\chi}_m(\omega) \approx \frac{2ic}{\sqrt{\tilde{\epsilon}_{ref}}\omega d}\ln\{\frac{\tilde{T}r_{ref}}{\tilde{T}r}\}. \tag{4}$$

# 10 THz frequency-domain measurements

THz frequency-domain spectroscopy (THz-FDS) was carried out using a frequency-tunable backward-wave-oscillator (BWO), generating continuous, coherent, and monochromatic THz radiation with a Golay cell serving as a detector and a He-bath cryostat for temperature control.[29] The transmittance was measured by recording the intensity of the THz radiation transmitted through the sample and referenced to the empty hole of the sample holder. Results are shown in **Figure S8**. In THz-FDS, a series of single frequency measurements were repeated to cover the frequency range between 7.5 to 13 cm$^{-1}$ which lacks the time resolution compared to the THz-TDS. Multiple reflections of the incident light between the parallel surfaces of transparent sample generate the pronounced Fabry-Perot oscillation pattern in Figure S8. In the THz-TDS, this effect can be avoided by controlling the time window. Nevertheless, the THZ-FDS measurements are in good qualitative agreement with the THZ-TDS results. Upon cooling to $T = 100$ K, the transmittance gets suppressed supporting the increase in the integrated absorption coefficient $IA$ for the in-plane orientation as presented in the main text (c.f. inset of Figure S8). From $T = 100$ K to $T = 20$ K, the transmittance rises again corresponding to a drop of the $IA$. Further cooling down to $T = 1.65$ K, a strong suppression of the transmittance is observed, in accordance with a rise of the $IA$ due to the excitations of the three-center magnon.

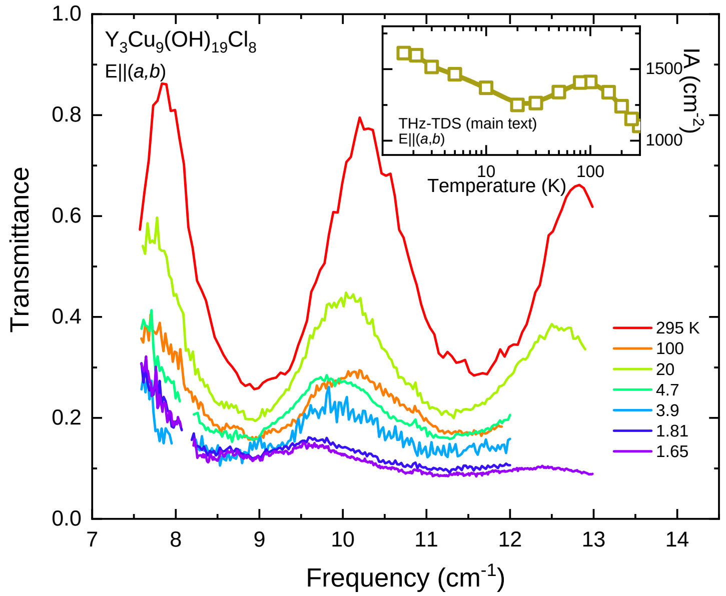


**Figure S8.** THz-FDS measurements. The temperature-dependent evolution of the transmittance is in good agreement with the $IA$ obtained by THZ-TDS (inset). The oscillation pattern in THz-FDS measurements originates from multiple internal reflections, as the transparent sample serves as a Fabry-Perot resonator, an etalon.

## 11 Magneto-optical THz-TDS

For magneto-optical THz-TDS measurements, a superconducting magnet (Oxford Instruments) is used to apply a static external magnetic field up to $H = 10$ T in Faraday geometry ($\boldsymbol{E}_{THz} \| (a,b)$, $\boldsymbol{H} \| c$) with temperature down to $T = 1.7$ K. **Figure S9** shows the time-domain electric fields and the corresponding absorption coefficient over the full magnetic field range. With increasing the magnetic field, the main pulse (below 4 ps) increases, while the extended-time oscillations lose intensity, c.f. Figure S9a. In the absorption coefficient, Figure S9b, this field dependency corresponds to a decrease of the continuum-like feature and the peak-like contributions between $30 - 40$ cm$^{-1}$ as expected from the spin-wave theory. As well, the phonon-tail (above 40 cm$^{-1}$) slightly shifts to lower frequencies.

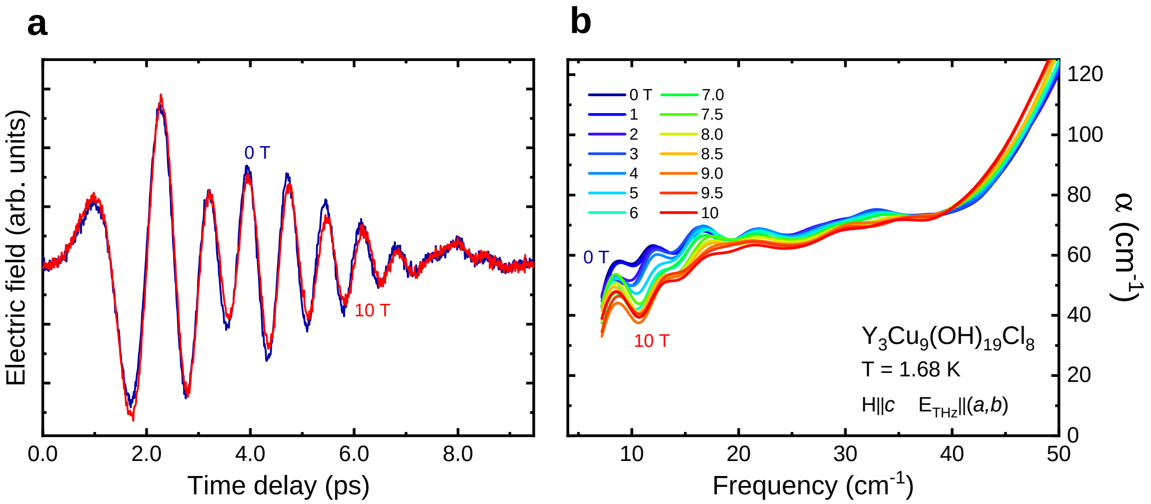


**Figure S9.** Magneto-optical THz-TDS result over the full magnetic field range. a,b) Time domain electric field and absorption coefficient in Faraday geometry ($\boldsymbol{E}_{THz} \parallel (a,b)$, $\boldsymbol{H} \parallel c$) at $T = 1.68$ K, respectively.

## 12 Details of the linear spin-wave theory calculations

We performed linear spin-wave theory (LSWT) to calculate the magnon dispersion and magnon density of states (shown in **Figure S10**) as implemented in SpinW 3.0.[30] The effective Hamiltonian for Y-kapellasite is given by a spin-1/2 Heisenberg Hamiltonian

$$H = \sum_{<i,j>} J_{i,j} \boldsymbol{S}_i \boldsymbol{S}_j, \tag{5}$$

where the sum goes over the first nearest neighbors (NN). The distortions in the lattice lead to three different NN couplings $J = 154.4$ K, $J_{\hexagon} = 134.2$ K, and $J' = 8.7$ K which have been calculated via DFT+U and the total energy mapping analysis.[31] The classical ground state was optimized by non-restricted energy optimization. The obtained classical ground state is given by a coplanar state with an ordering vector $\boldsymbol{Q} = (1/3, 1/3)$. The magnon energy dispersion is calculated on 1000 k-points along the path Γ-K-M-Γ as shown in the inset of the right panel in Figure S10. The magnon density of states is calculated on a 100×100×100 k-mesh by the definition

$$DOS(E) = \frac{1}{N} \sum_{i}^{N} \delta(E - E_i), \tag{6}$$

where $E$ is the energy and $E_i$ is the magnon energy with momentum $\mathbf{q}$. The Dirac delta function was approximated by a Lorentzian function

$$\delta_\epsilon(x) = \frac{1}{\pi} \frac{\epsilon}{x^2 + \epsilon^2}, \tag{7}$$

with $\epsilon = 0.01$ and energy resolution 0.01 meV.

## 13 Linear spin-wave theory calculations over an extended energy range

Figure S10 shows the spin dispersion and spin density of states (DOS) over an extended energy range obtained from linear spin-wave theory (LSWT). Besides the three-peak structure mentioned in the main text, there are several high-energy peaks in the DOS. For the comparison between the $\mathbf{q} = 0$ excitation and multi-center magnon excitation ($\Delta\mathbf{q} = 0$), we display the corresponding DOS curves ($\mathbf{q} = 0$ and over the entire Brillouin zone) in Figure S10 (left panel). The $\mathbf{q} = 0$ DOS mainly consists of three excitations ($E = 0$ meV Goldstone mode, around $E = 7.4$ meV, and $E = 8.4$ meV). Note that no excitations are expected in our experimental range (1 - 6 meV) within the $\mathbf{q} = 0$ limit which calls for the multi-center magnon picture facilitating the $\Delta\mathbf{q} = 0$ process. The latter two, $\mathbf{q} = 0$ magnons, $E = 7.4$ meV and $E = 8.4$ meV, are located in the energy-range of the far-infrared phonon modes, which might be related to spin-phonon coupling as suggested in main text.

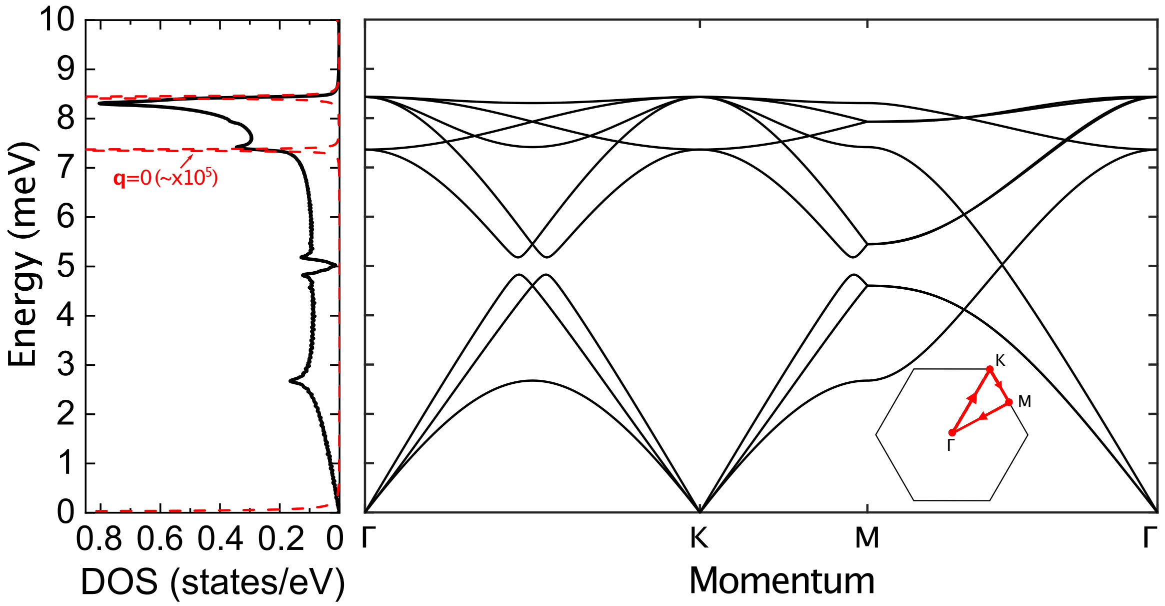


**Figure S10.** LSWT calculations. Left panel: DOS, black line: Integrated over the full Brillouin zone and red dashed line: $\mathbf{q} = 0$ contribution (scaled by a factor of $\sim 10^5$). Right panel: LSWT dispersion over an extended energy range. The inset shows the first Brillouin zone. The magnon dispersion has been calculated along the red arrows.

## 14 Calculation of $\chi_m''$

To confirm the spectral shape of the multi-center magnon and further compare directly between experiment and theory, we compute the imaginary part of the frequency-dependent magnetic susceptibility $\chi_m'' = \mathrm{Im}\{\tilde{\chi}_m(\omega)\}$ expected for the multi-center magnon absorption using the following relation [32]

$$\mathrm{Im}\{\tilde{\chi}_m(\omega)\} = \gamma \sum_q \sum_{\alpha,\beta} h_\alpha h_\beta \mathrm{Im}\{\chi^{SS}_{\alpha,\beta}(q,\omega)\}, \quad (8)$$

where $\gamma$ is a constant, $q$ is the momentum in the extended Brillouin zone, the summation $\alpha$ and $\beta$ goes over the Cartesian components, $\chi^{SS}_{\alpha,\beta}(q,\omega)$ is the spin susceptibility, and $h$ is the orientation of the THz magnetic field. At zero temperature the imaginary part of the spin susceptibility is related to the spin-spin correlation function $S_{\alpha,\beta}$:

$$\mathrm{Im}\{\chi^{SS}_{\alpha,\beta}(q,\omega)\} = S_{\alpha,\beta}(q,\omega), \quad (9)$$

where the spin-spin correlation function is computed within the SpinW 3.0 frame work. [30] The energy resolution of $\mathrm{Im}\{\tilde{\chi}_m(\omega)\}$ is 0.1 meV with broadening of 0.1.

Results are shown in **Figure S11**. As discussed in the main text, the experimental and theoretical energy scales are slightly shifted with respect to each other (about 1 meV). In the calculation, a pronounced, asymmetric peak (at around 2.7 meV), corresponding to the first peak in SDOS (same energy) is well-reproduced. Comparing within the experimentally accessible range, the overall shape shows a nice agreement including the double peak/ dip-like structure (around 4 to 4.6 meV in experiment, 5 meV in calculation) validating the multi-magnon scenario once more. The calculation shows a low-energy contribution (below 2 meV). This feature is outside our experimental range, but perhaps the extra broadening of the experimental peak might already contain the effect of this contribution.

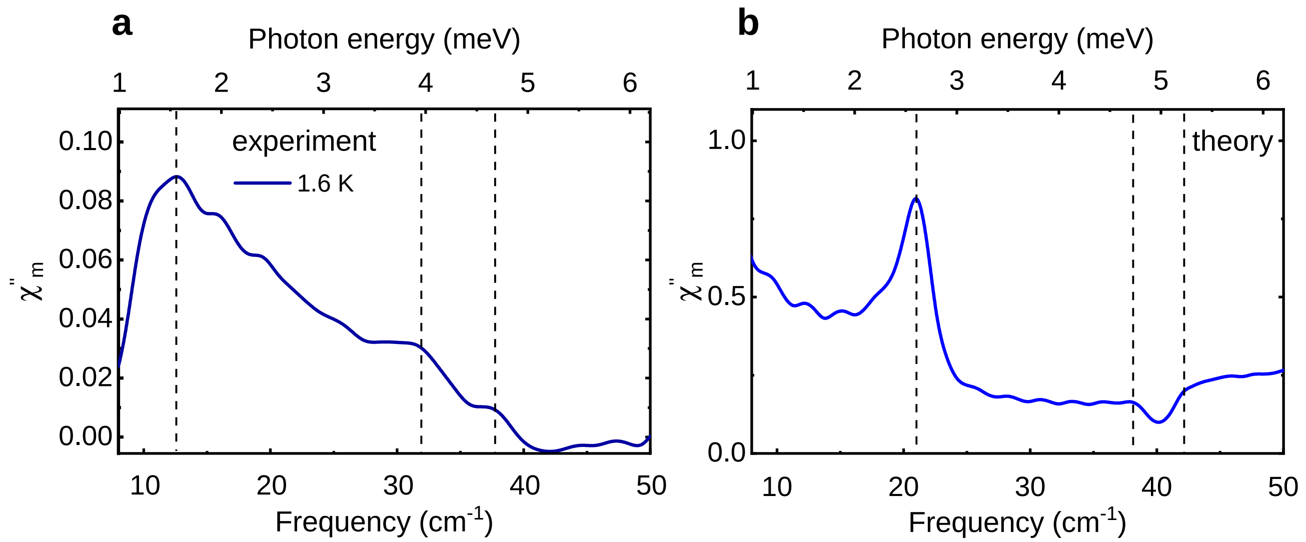


**Figure S11.** Comparison between (a) experimentally and (b) theoretically determined dynamic magnetic susceptibility $\chi_m''$. All experimental features are reproduced by the calculation. Note that the energy scale between experiment and theory is shifted by a small offset of about 1 meV.

## 15 Linear spin-wave theory calculations under magnetic field

**Figure S12** shows the calculated spin dispersion under external magnetic field. With increasing magnetic fields, the low-energy dispersion (0 to 3 meV) becomes gapped at the Γ and $K$ points and shifts to higher energies, partially lifting the degeneracy of the three lowest magnon bands. As well, shifts of the characteristic energy scales (between 3 and 6 meV, colored dashed lines), discussed in the main text, to higher energies are observable.

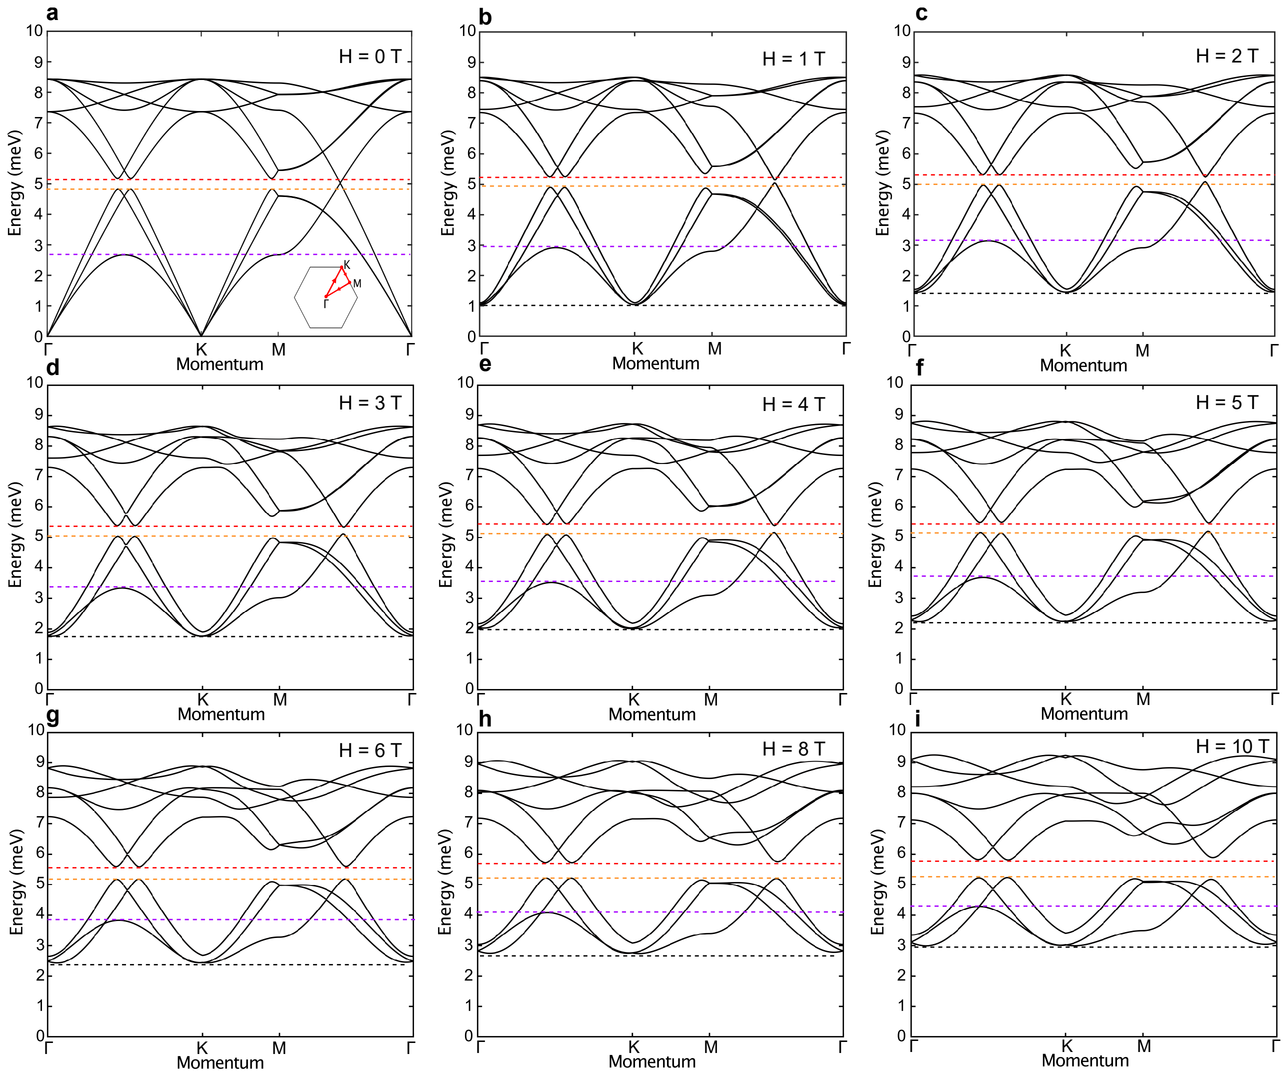


**Figure S12.** LSWT calculations with magnetic field. a-i) Dispersion in the first Brillouin zone (see inset of (a) for calculated path) with selected magnetic fields. Characteristic energy scales, discussed in the main text, are highlighted by colored dashed lines. Black dashed line: Minima of the Γ and $K$ points.

The corresponding SDOS is shown in **Figure S13**. Here, the shifting of the weight to higher energies for increased magnetic field is evident. In addition to the discussion in the main text, we discuss the changes at the higher energies (between 6 and 10 meV). At $H = 0$ the SDOS shows a sharp peak at around 8.3 meV. Under magnetic field the peak gets suppressed and its weight gets distributed over a larger energy range leading to an increase of the SDOS at around 6.8 meV / 55 cm$^{-1}$, i.e. the range of the lowest phonon tail. This field evolution might explain the shift of the phonon tail under magnetic field to lower energies, as observed in the magneto-THz experiment (main text).

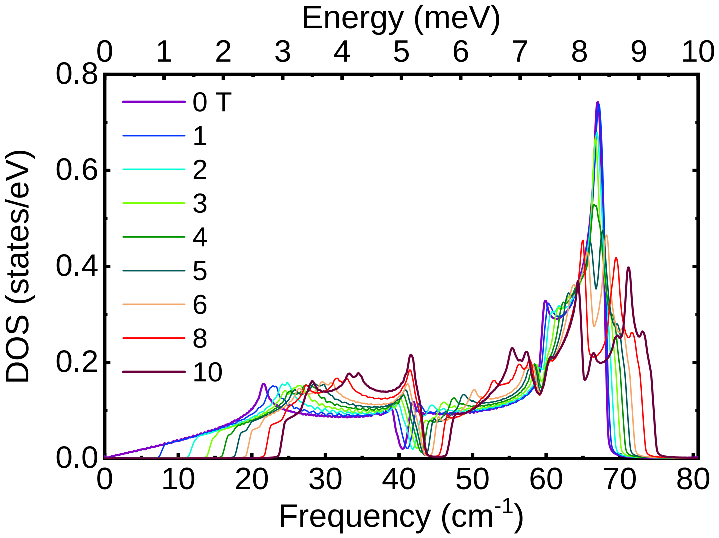


**Figure S13.** SDOS with magnetic field. Under magnetic field the SDOS becomes gapped and weight shifts to higher energies. Furthermore, between 6 and 10 meV, the weight gets distributed over a wider energy range.

## 16 Two-center magnon and three-center magnon excitation

For multi-center magnon absorption, i.e. the simultaneous flip of multiple spins by one photon, possible absorption can be either two-center or three-center magnon excitations. For each case, we consider the spin selection rule for linearly polarized THz light ($\Delta S = 0$[33,34]) in the magnetic ground state of Y-kapellasite. The two-center magnon excites two magnons simultaneously (left panel of **Figure S14**). Two scenarios are considered: two magnon excitations in one hexagon or two magnon excitations in different hexagons. Within a single hexagon, the $\Delta S = 0$ selection rule is satisfied if two spins of opposite sign are flipped simultaneously. However, excitations comprising two different hexagons are forbidden. Here, the non-collinearity of the magnetic ground state results in $\Delta S = \pm 1$. For the three-center magnon, the situation is reversed (right panel of Figure S14). Three spin flips inside a single hexagon cannot satisfy the selection rule but result in spin momentum changes of higher order. However, if one spins in each of the three different hexagons is flipped, the net spin momentum does not change. Therefore, for linearly polarized light the spin selection rule allows two cases: two-center magnon in one hexagon or three-center magnon that involves three different hexagons. Between these two, flipping one spin in each hexagon (three-center magnon) seems to be energetically more favorable. Our high-field magnetization experiment supports this idea by showing a 1/6 plateau. Hence, three-center magnon, involving one spin-flip in each of the three different hexagon, is most likely the main contribution of the THz absorption. In order to fully exclude contributions from the spin-allowed two-center process, complete theoretical considerations of the involved selection rules are necessary. This remains the focus of a future study.

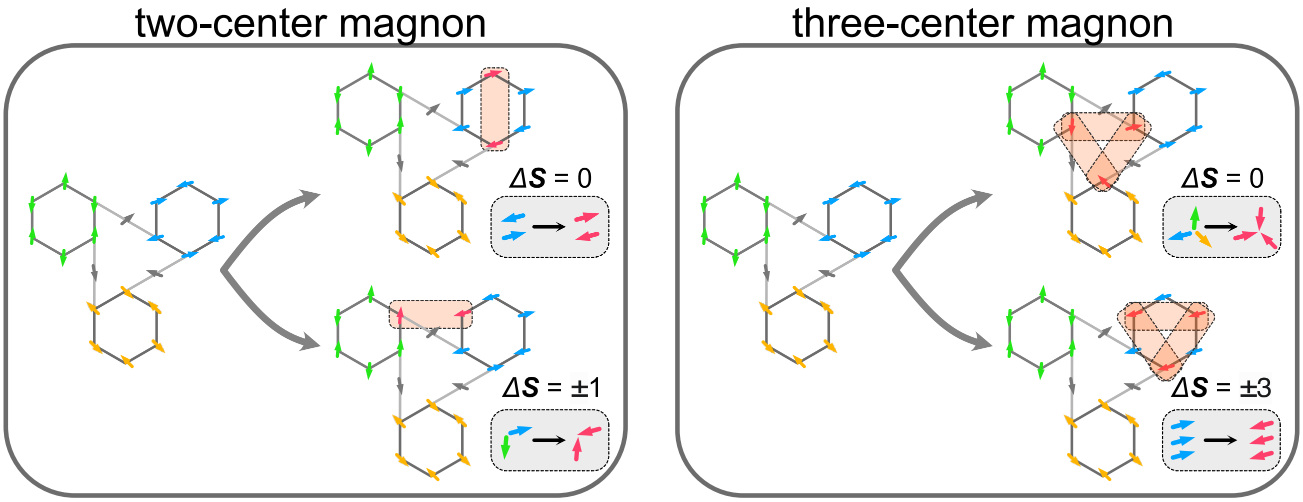


**Figure S14.** Possible multi-center magnon absorptions: two-center and three-center magnon in Y-kapellasite. Left panel: two-center magnon (red-shaded area) involving the simultaneous creation of two magnons (spin flips, grey-shaded inset) in one hexagon with $\Delta S = 0$ or a creation of two magnons in two different hexagons, $\Delta S = \pm 1$. Right panel: three-center magnon. Here, the creation of three magnons in three different hexagons gives $\Delta S = 0$, whereas three magnons in the same hexagons yield $\Delta S = \pm 3$. Note that for the $\Delta S = \pm 1$ / $\Delta S = \pm 3$ cases only one of the two possible spin-flip pictures is sketched.

## 17 Comparison with Herbertsmithite

THz-TDS was carried out on Herbertsmithite ($ZnCu_3(OH)_6Cl_2$). The transmitted time-domain electric fields ($\boldsymbol{E}_{THz} \parallel (a, b)$) are displayed in **Figure S15**a. Figure S15b shows corresponding absorption coefficient $\alpha$. The integrated absorption coefficient $IA$ is shown in Figure S15c. At room temperature, the absorption coefficient is dominated by the tail of the lowest in-plane phonon mode (around 85 $cm^{-1}$ [12]). Upon cooling the phonon shifts to higher energies, leading to a decrease of the $IA$. However, below $T = 50$ K, the $IA$ slightly increases again, similar to the previous report.[35] At low frequencies, we observe a monotonic response. As well, pronounced extended-time oscillations of the electric field are absent (Figure S15a). These observations are in stark contrast to the measurements on Y-kapellasite (see main text). Overall, our THz setup succesfully reproduced the previous results on Herbertsmithite (Reference[35]), supporting that all differences between Y-kapellasite and Herbertsmithite THz spectra are due to the different magnetic ground states.

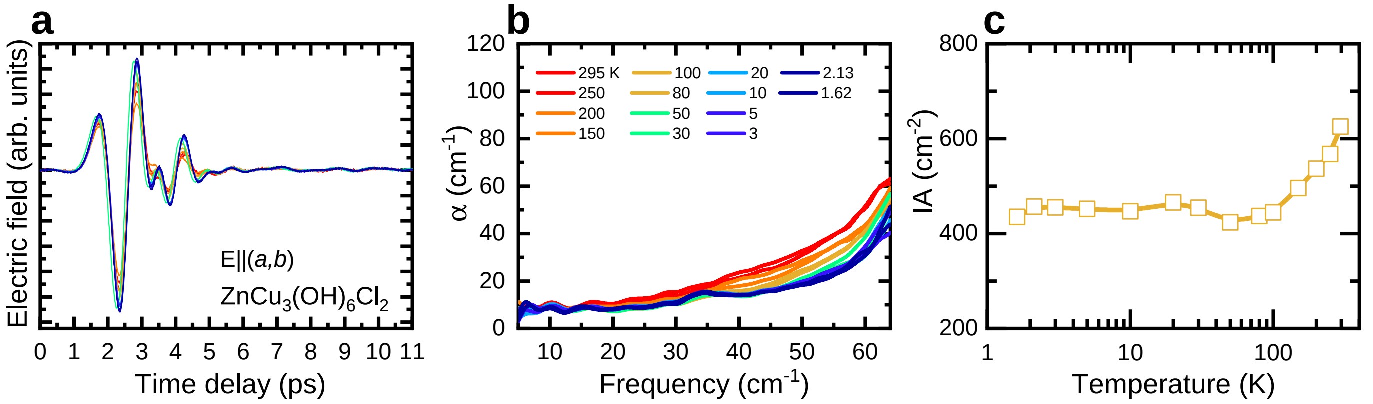


**Figure S15.** THZ-TDS on $ZnCu_3(OH)_6Cl_2$. a,b) Time domain electric field and absorption coefficient for the in-plane $\boldsymbol{E} \parallel (a, b)$ response, respectively. c) Integrated absorption coefficient $IA$ (up to 46 $cm^{-1}$).

## References

[S1] P. Puphal, M. Bolte, D. Sheptyakov, A. Pustogow, K. Kliemt, M. Dressel, M. Baenitz, C. Krellner, *J. Mater. Chem. C* **2017**, *5* 2629.

[S2] Q. Barthélemy, P. Puphal, K. M. Zoch, C. Krellner, H. Luetkens, C. Baines, D. Sheptyakov, E. Kermarrec, P. Mendels, F. Bert, *Phys. Rev. Mater.* **2019**, *3* 074401.

[S3] W. Sun, T. Arh, M. Gomilšek, P. Koželj, S. Vrtnik, M. Herak, J.-X. Mi, A. Zorko, *Phys. Rev. Mater.* **2021**, *5* 064401.

[S4] W. Sun, Y.-X. Huang, S. Nokhrin, Y. Pan, J.-X. Mi, *J. Mater. Chem. C* **2016**, *4* 8772.

[S5] R. T. Schumacher, C. P. Slichter, *Phys. Rev.* **1956**, *101* 58.

[S6] Y. Skourski, M. D. Kuz'min, K. P. Skokov, A. V. Andreev, J. Wosnitza, *Phys. Rev. B* **2011**, *83* 214420.

[S7] Y. Kohama, H. Ishikawa, A. Matsuo, K. Kindo, N. Shannon, Z. Hiroi, *Proc. Natl. Acad. Sci. U.S.A.* **2019**, *116*, 22 10686.

[S8] O. Janson, S. Furukawa, T. Momoi, P. Sindzingre, J. Richter, K. Held, *Phys. Rev. Lett.* **2016**, *117* 037206.

[S9] C. C. Homes, M. Reedyk, D. A. Cradles, T. Timusk, *Appl. Opt.* **1993**, *32*, 16 2976.

[S10] M. Dressel, A. Pustogow, *J. Phys. Condens. Matter* **2018**, *30*, 20 203001.

[S11] D. B. Tanner, *Optical Effects in Solids*, Cambridge University Press, Cambridge, **2019**.

[S12] Y. Li, A. Pustogow, M. Bories, P. Puphal, C. Krellner, M. Dressel, R. Valentí, *Phys. Rev. B* **2020**, *101* 161115.

[S13] I. I. Mazin, *Phys. Rev. B* **2010**, *81* 140508.

[S14] R. D. Johnson, I. Broeders, K. Mehlawat, Y. Li, Y. Singh, R. Valentí, R. Coldea, *Phys. Rev. B* **2019**, *100* 214113.

[S15] A. Togo, F. Oba, I. Tanaka, *Phys. Rev. B* **2008**, *78* 134106.

[S16] A. Togo, I. Tanaka, *Scr. Mater.* **2015**, *108* 1.

[S17] K. Parlinski, Z. Q. Li, Y. Kawazoe, *Phys. Rev. Lett.* **1997**, *78* 4063.

[S18] J. P. Perdew, K. Burke, M. Ernzerhof, *Phys. Rev. Lett.* **1996**, *77* 3865.

[S19] G. Kresse, J. Hafner, *Phys. Rev. B* **1993**, *47* 558.

[S20] G. Kresse, J. Furthmüller, *Phys. Rev. B* **1996**, *54* 11169.

[S21] G. Kresse, J. Furthmüller, *Comput. Mater. Sci.* **1996**, *6*, 1 15.

[S22] K. Kozuki, T. Nagashima, M. Hangyo, *Opt. Express* **2011**, *19*, 25 24950.

[S23] L. Pan, N. J. Laurita, K. A. Ross, B. D. Gaulin, N. P. Armitage, *Nat. Phys.* **2016**, *12*, 4 361.

[S24] X. Zhang, F. Mahmood, M. Daum, Z. Dun, J. A. M. Paddison, N. J. Laurita, T. Hong, H. Zhou, N. P. Armitage, M. Mourigal, *Phys. Rev. X* **2018**, *8* 031001.

[S25] N. J. Laurita, J. Deisenhofer, L. Pan, C. M. Morris, M. Schmidt, M. Johnsson, V. Tsurkan, A. Loidl, N. P. Armitage, *Phys. Rev. Lett.* **2015**, *114* 207201.

[S26] N. J. Laurita, G. G. Marcus, B. A. Trump, J. Kindervater, M. B. Stone, T. M. McQueen, C. L. Broholm, N. P. Armitage, *Phys. Rev. B* **2017**, *95* 235155.

[S27] P. Chauhan, F. Mahmood, H. J. Changlani, S. M. Koohpayeh, N. P. Armitage, *Phys. Rev. Lett.* **2020**, *124*, 3 037203.

[S28] M. Dressel, G. Grüner, *Electrodynamics of Solids: Optical Properties of Electrons in Matter*, Cambridge University Press, Cambridge, **2002**.

[S29] U. S. Pracht, E. Heintze, C. Clauss, D. Hafner, R. Bek, D. Werner, S. Gelhorn, M. Scheffler, M. Dressel, D. Sherman, B. Gorshunov, K. S. Il'in, D. Henrich, M. Siegel, *IEEE Trans. Terahertz Sci. Technol.* **2013**, *3*, 3 269.

[S30] S. Toth, B. Lake, *J. Phys. Condens. Matter* **2015**, *27*, 16 166002.

[S31] M. Hering, F. Ferrari, A. Razpopov, I. I. Mazin, R. Valentí, H. O. Jeschke, J. Reuther, *Npj Comput. Mater.* **2022**, *8*, 1 10.

[S32] R. S. Fishman, J. A. Fernandez-Baca, T. Rõõm, *Spin-Wave Theory and its Applications to Neutron Scattering and THz Spectroscopy*, Morgan & Claypool Publishers, San Rafael, **2018**.

[S33] C. Cohen-Tannoudji, B. Diu, F. Laloë, *Quantum Mechanics VOL 2 2ed*, Wiley, New York, **2019**.

[S34] C. Cohen-Tannoudji, B. Diu, F. Laloë, *Quantum Mechanics VOL 3 2ed*, Wiley, New York, **2020**.

[S35] D. V. Pilon, C. H. Lui, T.-H. Han, D. Shrekenhamer, A. J. Frenzel, W. J. Padilla, Y. S. Lee, N. Gedik, *Phys. Rev. Lett.* **2013**, *111* 127401.
